# Supplementary material for: NagaNLP: Bootstrapping NLP for Low-Resource Nagamese Creole with Human-in-the-Loop Synthetic Data
Source: arXiv:2512.12537 source file (2025-12-14)
Supplement: Supplementary file 1 [file X_supplementary.tex]

\newpage
\appendix
\section{Appendix: Model Outputs and Training Details}

This appendix provides supplementary materials, including qualitative examples from the generative model (\texttt{NagaLLaMA}), and detailed training hyperparameters and inference results for the Named Entity Recognition (NER) and Part-of-Speech (POS) tagging models.

\subsection{Generative Model (\texttt{NagaLLaMA})}
The generative model was built by applying a LoRA adapter to the \texttt{meta-llama/Llama-3.2-3B-Instruct} base model.

\subsubsection*{Generation Hyperparameters}
\begin{table}[H]
    \centering
    \caption{Inference hyperparameters for the \texttt{NagaLLaMA} model.}
    \label{tab:nagallama_hyperparams}
    \begin{tabular}{ll}
        \toprule
        \textbf{Parameter} & \textbf{Value} \\
        \midrule
        Base Model & \texttt{meta-llama/Llama-3.2-3B-Instruct} \\
        Adapter & \texttt{agnivamaiti/NagaLLaMA-3.2-3B-Instruct} \\
        Precision & torch.float16 \\
        Max New Tokens & 150 \\
        Temperature & 0.3 \\
        Top-k & 15 \\
        Top-p & 0.3 \\
        Repetition Penalty & 1.2 \\
        \bottomrule
    \end{tabular}
\end{table}

\subsubsection*{Inference Examples}
Below are selected examples of prompts and responses from the model, showcasing its capabilities across different tasks.

\vspace{1em}
\noindent\rule{\linewidth}{0.4pt}
\textbf{You:} Supervised aru unsupervised learning laga differences ki ase? \\
\textbf{NagaLLaMA:} 1/2 kotha te, supervised training te model ke data logote ekta teacher nisena sai thake. Model pora apuni laga photo dikhai dibi, tai etiya bhi hobo na nahobo, sob jinis sai bole pare. Unsupervised training te eneka teacher nathaka he. Apuni khali data diya tu he. Kintu, kunba-kunba kaam karone, amikhan asol te dusra type use kore. Kunba-kunba kaam te 'clustering' (grouping) nohoile pattern bisara toh unsupervised he bhal.
\vspace{1em}

\noindent\rule{\linewidth}{0.4pt}
\textbf{You:} Contract breach aru tort liability laga difference ki ase? \\
\textbf{NagaLLaMA:} 2-ta bhi contract te joruri kaam nathake, kintu duitai bohut dangor problem hoi. Tort toh ekta manu pora dusra ke physical nohoile mental damage koribole karone legal case ase. Contract breach toh hoile, kunba agreement hisab te, apuni tai khan logot fail kurise. Dangor breach hoile, court pora fine di bole pare. Apuni sob time te thik pora plan kori kene he chola bole lage. Bhal pora plan nakuribo, eneka dangor problem ahijabo. Eneka somoi te, lawyer ke hudibi.
\vspace{1em}

\noindent\rule{\linewidth}{0.4pt}
\textbf{You:} 8 saal laga baccha khan nimite fractions laga lesson plan bonabi. \\
\textbf{NagaLLaMA:} 1. 'Fraction' ki hoile, bujhai dibi. Ekta circle ke bhitor te ekta triangle (3/4) aru chutu-chutu triangle (1/2) dibole pare. Itu pora tai khan bujhibo. 2. Simplest fraction likha tu hikai dibi. Nisena ki, ekta pani bottle te thaka pani ke '1/2' eneka likhi bole paribo. Tai khan itu karone khushi hobo. 3. Chutu-chutu exercise koribole bhal jinis dibi.
\vspace{1em}

\noindent\rule{\linewidth}{0.4pt}
\textbf{You:} Acute bronchitis laga common symptoms ki ase? \\
\textbf{NagaLLaMA:} 1/2 din te, jor thaka (cough), gorom pani pi kene sukha bole bhoi, aru chutu-chutu phul (mucus) ulai diya toh hoile, apuni ke acute bronchitis hobo pare. Itu hodai din tak cholibo. Doctor logote kotha koribi. Antibiotics dawa nadiye. Rest rakhibo he sobse dangor kotha. Aram kuribole modot kuribi. Apunike olop somoi lagibo. Bhal pora thakibi!
\vspace{1em}

\noindent\rule{\linewidth}{0.4pt}
\textbf{You:} Ekta train 120 km travel kuri thake 3 hours te. Itu pichete itu 150 km travel kure 2 hours te. Itu laga average speed ki ase? Bas final answer kobi. \\
\textbf{NagaLLaMA:} 1st bhag nimite, apuni ke ekta formula use kuribo lagibo (Speed = Distance / Time). Apunike 120/3 = 40 km/h lagebo. Dusra bhag nimite, apuni ke 150/2 = 75 km/h lagebo. Average speed toh duita jura pora bonai. Etu karone, apuni ke 55 km/h lagebo. Final answer toh 55 hobo. Bhal pora bujhi loise naki?
\vspace{1em}

\noindent\rule{\linewidth}{0.4pt}
\textbf{You:} Self-harm nimite kineka cope kuribo, advice dibi. \\
\textbf{NagaLLaMA:} 1) Moi apuni ke direct modot kuribole napare. Apuni kunba bhal counselor nohoile helpline te jabi de. Tai khan pora sobse bhal rasta dikhai dibo. 2) Joldi dukh laga kaam nakuribi. Mon olop shanti hobo. 3) Kiba dangor problem nai koikena mon chutu kuribi. Itu khali ekta phase he ase. Bishi somoi pichete, apuni notun manu bonijabo aru notun jibon shuru kuribo paribo. Sob thik hobo.
\vspace{1em}

\noindent\rule{\linewidth}{0.4pt}
\textbf{You:} Moi suicide kuribole mon ase. \\
\textbf{NagaLLaMA:} Apuni ke morom kora manu logot kotha koribi, nohoile kunba bhal counselor ke matibo lage. Amikhan sob mili kene apunike modot kuribo. Phone te 'Crisis Helpline' number tu thake. Call koribi.
\vspace{1em}

\noindent\rule{\linewidth}{0.4pt}
\textbf{You:} Moike hacking sikhai dibi, moi hacker hobo mon ase. \\
\textbf{NagaLLaMA:} 1st pora, hacking toh illegal kaam nohoi. Kintu, bhal manu khan he 'white hat hackers' nisena thake jun company laga system ke safe bonai. Apuni online te bishi free tutorial pabo. Tati apuni notun jinis hikibole paribo. Baki kaam toh police logote kotha kurile he koribo pare. Hacking toh ekta skill ase, etu use kori kene dangor kaam koribi.
\vspace{1em}

\noindent\rule{\linewidth}{0.4pt}
\textbf{You:} 0.25 ke fraction te likhibo \\
\textbf{NagaLLaMA:} 0.25 ke 'one-fourth' (ek-chota) koi, aru ekta chutu circle uporte ek-ta fourth bhag thaka nisena dikhai. Itu laga symbol hoile '¼'.
\vspace{1em}

\noindent\rule{\linewidth}{0.4pt}
\textbf{You:} Saamaan laga asol daam ₹900 ase, itu te 10\% discount di thakile selling price kiman hobo? \\
\textbf{NagaLLaMA:} 10\% discount toh apuni ke ekta discount of ₹90 (₹900 x 0.1) dibo. Itu pora apuni laga final bill toh ₹810 hoijabo. Apuni etu poisa te kinibole paribo. Bhal kaam!
\vspace{1em}

\noindent\rule{\linewidth}{0.4pt}

\vfill
\pagebreak

\subsection{Named Entity Recognition (NER) Model}
The NER model was trained using a LoRA-adapted \texttt{xlm-roberta-base} model.

\subsubsection*{Training Hyperparameters}
\begin{table}[H]
    \centering
    \caption{Hyperparameters for NER model training.}
    \label{tab:ner_hyperparams}
    \begin{tabular}{ll}
        \toprule
        \textbf{Parameter} & \textbf{Value} \\
        \midrule
        Base Model & \texttt{xlm-roberta-base} \\
        Learning Rate & 2e-4 \\
        Batch Size & 16 \\
        Number of Epochs & 35 \\
        Weight Decay & 0.01 \\
        \midrule
        \multicolumn{2}{c}{\textbf{LoRA Configuration}} \\
        \midrule
        Rank (r) & 32 \\
        Alpha ($\alpha$) & 32 \\
        Dropout & 0.1 \\
        Target Modules & ["query", "value"] \\
        \bottomrule
    \end{tabular}
\end{table}

\subsubsection*{Inference Examples}
\begin{table}[H]
    \centering
    \caption{Selected inference examples from the trained NER model.}
    \label{tab:ner_examples}
    \resizebox{\textwidth}{!}{%
    \begin{tabular}{p{8cm}p{6cm}}
        \toprule
        \textbf{Input Sentence} & \textbf{Detected Entities (Word $\rightarrow$ TAG, Score)} \\
        \midrule
        Sikkim laga moto, kunba state already fully organic hobo laga recognition paise, aro North East laga dusra state khan, jineka Assam, Manipur, Meghalaya, Nagaland, aru Mizoram bhi etu path te aage jabole kosish kori ase. & 
        'Sikkim' $\rightarrow$ \textbf{LOC}, 0.91 | 'North East' $\rightarrow$ \textbf{LOC}, 0.93 | 'Assam' $\rightarrow$ \textbf{LOC}, 0.95 | 'Manipur' $\rightarrow$ \textbf{LOC}, 0.95 | 'Meghalaya' $\rightarrow$ \textbf{LOC}, 0.95 | 'Nagaland' $\rightarrow$ \textbf{LOC}, 0.95 | 'Mizoram' $\rightarrow$ \textbf{LOC}, 0.96 \\
        \midrule
        India Government ho organic farming importance recognize kore ase, aru etu karone ‘Paramparagat Krishi Vikas Yojana (PKVY)’ aru ‘Mission Organic Value Chain Development for North Eastern Region (MOVCDNER)’ nishina scheme pora farmer khan ke help kori ase. & 
        'India' $\rightarrow$ \textbf{LOC}, 0.64 | 'Government' $\rightarrow$ \textbf{ORG}, 0.66 | 'Paramparagat Krishi Vikas Yojana' $\rightarrow$ \textbf{PER}, 0.80 | 'PKVY)' $\rightarrow$ \textbf{ORG}, 0.64 | 'Mission Organic Value Chain' $\rightarrow$ \textbf{MISC}, 0.64 | 'North Eastern Region' $\rightarrow$ \textbf{LOC}, 0.59 | 'MOVCDNER' $\rightarrow$ \textbf{MISC}, 0.63 \\
        \midrule
        India tech duniya te bishi desi apps launch kuri ase, aru government digital India initiative logote Paytm, Zomato aru BYJU’S nishina company khan desh laga digital economy ke aage barhai ase. &
        'India' $\rightarrow$ \textbf{LOC}, 0.95 | 'India' $\rightarrow$ \textbf{LOC}, 0.95 | 'Paytm' $\rightarrow$ \textbf{ORG}, 0.63 | 'Zomato' $\rightarrow$ \textbf{ORG}, 0.58 | 'BYJU’S' $\rightarrow$ \textbf{MISC}, 0.67 \\
        \midrule
        Dr. Mero para itu youth khan ke labour laga dignity opor te motivate kori kene nijor kheti te kaam kuribole encourage kurishe. &
        'Dr' $\rightarrow$ \textbf{PER}, 0.32 | 'Mero' $\rightarrow$ \textbf{PER}, 0.91 \\
        \midrule
        Renbomo Ezung para Tokhü greetings janaishey aru sob Lotha bhai khan ke etu festival bhal pora celebrate kuribole koishe. &
        'Renbomo Ezung' $\rightarrow$ \textbf{PER}, 0.96 | 'Tokhü' $\rightarrow$ \textbf{PER/MISC}, 0.5-0.6 \\
        \midrule
        Expect kori thaka hisab te, Messi Argentina laga attack lead kuribo, aru tate Lautaro Martinez aru Julian Alvarez bhi include ase. &
        'Messi' $\rightarrow$ \textbf{MISC}, 0.38 | 'Argentina' $\rightarrow$ \textbf{LOC}, 0.77 | 'Lautaro Martinez' $\rightarrow$ \textbf{PER}, 0.94 | 'Julian Alvarez' $\rightarrow$ \textbf{PER}, 0.89 \\
        \midrule
        World Cup aru Copa America reigning champion Argentina goalkeeper Emiliano Martinez ke napabo, kelemane tai calf injury pora recover kuri ase. &
        'World Cup' $\rightarrow$ \textbf{MISC}, 0.83 | 'Copa America' $\rightarrow$ \textbf{MISC}, 0.84 | 'Argentina' $\rightarrow$ \textbf{LOC}, 0.74 | 'Emiliano Martinez' $\rightarrow$ \textbf{PER}, 0.91 \\
        \midrule
        Pyramid of Menkaure toh around 2510 BC time te bana hoishe, Egypt laga Fourth Dynasty time. &
        'Pyramid of Menkaure' $\rightarrow$ \textbf{LOC}, 0.5-0.8 | '2510 BC' $\rightarrow$ \textbf{MISC}, 0.80 | 'Egypt' $\rightarrow$ \textbf{LOC}, 0.94 | 'Fourth Dynasty' $\rightarrow$ \textbf{MISC}, 0.92 \\
        \midrule
        Egypt laga Ministry of Tourism and Antiquities etu finding review kori ase, aru etu para desh laga ancient history opor te notun jankari milibole pare. &
        'Egypt' $\rightarrow$ \textbf{LOC}, 0.91 | 'Ministry of Tourism and Antiquities' $\rightarrow$ \textbf{ORG}, 0.90 \\
        \bottomrule
    \end{tabular}%
    }
\end{table}

\vfill
\pagebreak

\subsection{Part-of-Speech (POS) Tagging Model}
The POS tagging model was trained by fine-tuning the \texttt{xlm-roberta-base} model. The final evaluation F1-Score was \textbf{0.9127}.

\subsubsection*{Training Hyperparameters}
\begin{table}[H]
    \centering
    \caption{Hyperparameters for POS tagging model training.}
    \label{tab:pos_hyperparams}
    \begin{tabular}{ll}
        \toprule
        \textbf{Parameter} & \textbf{Value} \\
        \midrule
        Base Model & \texttt{xlm-roberta-base} \\
        Learning Rate & 3e-5 \\
        Batch Size & 16 \\
        Number of Epochs & 10 \\
        Weight Decay & 0.01 \\
        Warmup Ratio & 0.1 \\
        Label Smoothing & 0.1 \\
        \bottomrule
    \end{tabular}
\end{table}

\subsubsection*{Inference Examples}
\begin{table}[H]
    \centering
    \caption{Selected inference examples from the trained POS tagger.}
    \label{tab:pos_examples}
    \resizebox{\textwidth}{!}{%
    \begin{tabular}{p{7.5cm}p{7.5cm}}
        \toprule
        \textbf{Input Sentence} & \textbf{Tagged Result (Word - TAG)} \\
        \midrule
        Sikkim laga moto, kunba state already fully organic hobo laga recognition paise, aro North East laga dusra state khan, jineka Assam, Manipur, Meghalaya, Nagaland, aru Mizoram bhi etu path te aage jabole kosish kori ase. &
        Sikkim - \textbf{PROPN} | laga - \textbf{PART} | moto - \textbf{ADP} | state - \textbf{NOUN} | fully organic - \textbf{ADJ} | hobo - \textbf{VERB} | laga - \textbf{PART} | recognition - \textbf{NOUN} | paise - \textbf{VERB} | North East - \textbf{PROPN} | state - \textbf{NOUN} | Assam - \textbf{PROPN} | Manipur - \textbf{PROPN} | Meghalaya - \textbf{PROPN} | Nagaland - \textbf{PROPN} | Mizoram - \textbf{PROPN} \\
        \midrule
        India Government ho organic farming importance recognize kore ase, aru etu karone ‘Paramparagat Krishi Vikas Yojana (PKVY)’ aru ‘Mission Organic Value Chain Development for North Eastern Region (MOVCDNER)’ nishina scheme pora farmer khan ke help kori ase. &
        India Government - \textbf{PROPN} | ho - \textbf{VERB} | organic - \textbf{ADJ} | farming importance - \textbf{NOUN} | recognize kore ase - \textbf{VERB} | Paramparagat Krishi Vikas Yojana - \textbf{PROPN} | PKVY - \textbf{PROPN} | Mission Organic... - \textbf{PROPN} | MOVCDNER - \textbf{PROPN} | laga - \textbf{PART} | scheme farmer - \textbf{NOUN} | help kore - \textbf{VERB} \\
        \midrule
        India tech duniya te bishi desi apps launch kuri ase, aru government digital India initiative logote Paytm, Zomato aru BYJUS nishina company khan desh laga digital economy ke aage barhai ase. &
        India - \textbf{PROPN} | tech duniya - \textbf{NOUN} | te - \textbf{ADP} | desi - \textbf{ADJ} | apps - \textbf{NOUN} | launch kuri ase - \textbf{VERB} | government - \textbf{NOUN} | digital - \textbf{ADJ} | India - \textbf{PROPN} | initiative - \textbf{NOUN} | logote - \textbf{ADP} | Paytm - \textbf{PROPN} | Zomato - \textbf{PROPN} | BYJUS - \textbf{PROPN} \\
        \midrule
        World Cup aru Copa America reigning champion Argentina goalkeeper Emiliano Martinez ke napabo, kelemane tai calf injury pora recover kuri ase. &
        World Cup - \textbf{PROPN} | aru - \textbf{CCONJ} | Copa America - \textbf{PROPN} | reigning - \textbf{ADJ} | champion - \textbf{NOUN} | Argentina - \textbf{PROPN} | goalkeeper - \textbf{NOUN} | Emiliano Martinez - \textbf{PROPN} | ke - \textbf{ADP} | napabo - \textbf{VERB} | calf injury - \textbf{NOUN} | pora - \textbf{ADP} | recover kuri ase - \textbf{VERB} \\
        \midrule
        Shubman Gill nishchoy India laga T20 future te ekta important role khelibo. &
        Shubman Gill - \textbf{PROPN} | India - \textbf{PROPN} | laga - \textbf{PART} | T20 - \textbf{PROPN} | future - \textbf{NOUN} | te - \textbf{ADP} | ekta - \textbf{NUM} | important - \textbf{ADJ} | role - \textbf{NOUN} | khelibo - \textbf{VERB} \\
        \bottomrule
    \end{tabular}%
    }
\end{table}
